# Supplementary material for: MLIP-MC: A Framework for Adsorption Simulations using Machine-Learned Interatomic Potentials
Source: arXiv:2602.13725 ancillary file (2026-02-14)
Supplement: Supplementary file 1 [file SI.pdf]

# **Supplementary Information for “MLIP-MC: A Framework for Adsorption Simulations using Machine-Learned Interatomic Potentials”**

Connor W. Edwards, Fengxu Yang, Konstantin Stracke, and Jack D. Evans\*

*School of Physics, Chemistry and Earth Sciences, Adelaide University, South Australia  
5000, Australia*

E-mail: [j.evans@adelaide.edu.au](mailto:j.evans@adelaide.edu.au)

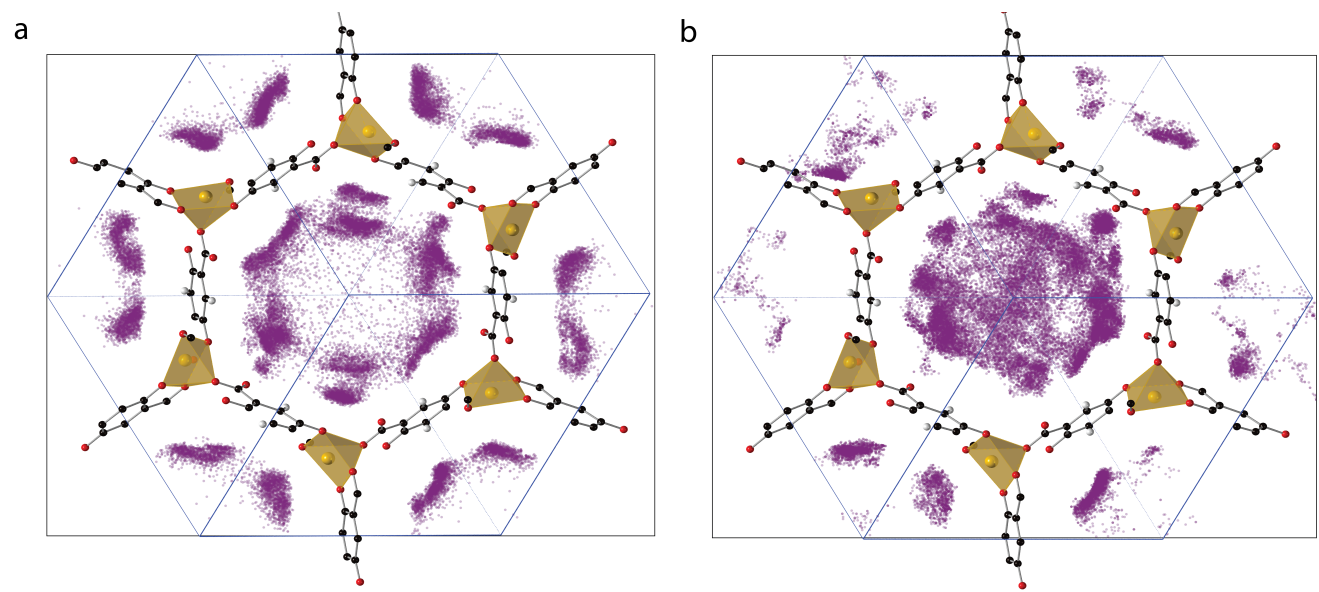

Supplementary Figure S1: Centre of mass of each CO<sub>2</sub> from 1 000 000 steps GCMC simulation of Mg-MOF-74 at a) 0.5 bar and b) 50 bar projected onto the XY plane. The structure of Mg-MOF-74 has been overlayed. Carbon is black, oxygen is red, hydrogen is white and Mg is yellow.

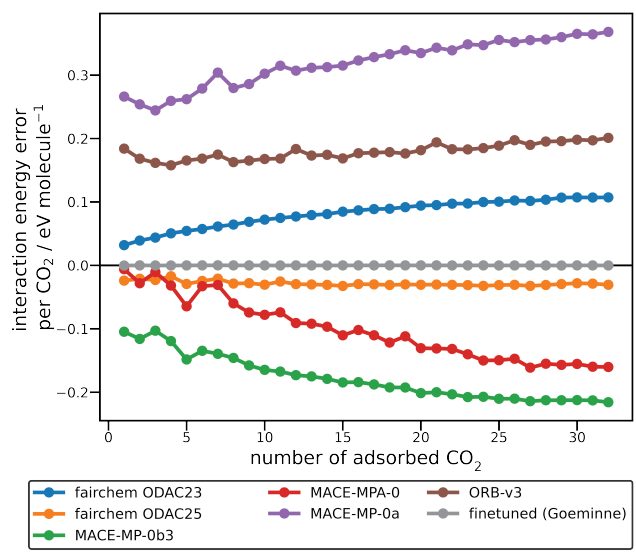

Supplementary Figure S2: Error in interaction energy per CO<sub>2</sub> for the adsorption on ZIF-8 predicted relative to the reference DFT reported by Goeminne et al.<sup>1</sup>

## References

- (1) Goeminne, R.; Vanduyfhuys, L.; Van Speybroeck, V.; Verstraelen, T. DFT-Quality Adsorption Simulations in Metal–Organic Frameworks Enabled by Machine Learning Potentials. *Journal of Chemical Theory and Computation* **2023**, *19*, 6313–6325.
